# Supplementary material for: AutoNet: Automatic Reachability Policy Management in Public Cloud Networks
Source: arXiv:2404.19372 source file (2024-04-30)
Supplement: Supplementary file 1 [file appendix.tex]

\appendix

\section{Network encoding algorithm}\label{app:linearity}
\cref{alg:encoding} describes a simplified version of the procedure used to perform the network reachability encoding in VARC. The procedure receives as input the network to be encoded and output the entire encoding. We define symbolic variables $s,d$ through the Z3 engine and use them to describe the overall reachability. The algorithm iterates over all subnets present in the topology and over all endpoints belonging ot each subnet. On \cref{lst:line:mapping_source_subnet} and \cref{lst:line:mapping_destination_subnet} we define the variables that hold the mapping between each endpoint and the corresponding subnet that are later updated on line \cref{lst:line:mapping_source_subnet_update}, and \cref{lst:line:mapping_destination_subnet_update} as a logical disjunction of all of the endpoints beloning to the subnet. Additionally, on line \cref{lst:line:intrasubnet_source_expression} and \cref{lst:line:intrasubnet_destination_expression} we build the expression related to the intra-subnet communication. The expression effectively forces the use of the endpoint-based reachability expression depending on the direction of the traffic flow. On \cref{lst:line:intersubnet_expression} we build the expression related to the inter-subnet communication. The expression forces the use use of subnet-based node filtering expressions only when a particular source and destination belong to different subnets (expressed by the exclusive or). Note that, for simplicity we i) limit the description of the algorithm to the VPC-level, i.e., we do not show the encoding in the case of multiple VPCs, and ii) we leave the details regarding the encoding of other network services such as ELB, EIP, NAT-GW etc. Nevertheless, the extension to the general case is trivial.
\begin{algorithm}[t]
   \caption{A simplified version of the network encoding algorithm used by VARC}
   \label{alg:encoding}
   \begin{algorithmic}[1]
      \Procedure{Encode}{Network}
      \State $s = \texttt{Sym("src node")}$ \Comment Symbolic source variable
      \State $d = \texttt{Sym("dst node")}$ \Comment Symbolic destination variable
      \State $R = \texttt{True}$
      \For{ $\texttt{subnet} \in \texttt{Network.Subnets}$}
         \State $M^{(E)} = \texttt{False}$ \label{lst:line:mapping_source_subnet}
         \State $M^{(I)} = \texttt{False}$ \label{lst:line:mapping_destination_subnet}
         \State $\texttt{IntraSubnet} = \texttt{True}$
         \For{ $\texttt{endpoint} \in \texttt{subnet}$}
            \State $M^{(E)} = M^{(E)} \vee (s = \texttt{endpoint.id})$ \label{lst:line:mapping_source_subnet_update}
            \State  $M^{(I)} = M^{(E)} \vee (d = \texttt{endpoint.id})$ \label{lst:line:mapping_destination_subnet_update}
            \State $ \texttt{IntraSubnet} = \texttt{IntraSubnet} \wedge ((d = \texttt{endpoint.id}) \rightarrow R_{endpoint}^{(I)})$ \label{lst:line:intrasubnet_source_expression}
            \State $\texttt{IntraSubnet} = \texttt{IntraSubnet} \wedge ((s = \texttt{endpoint.id}) \rightarrow R_{endpoint}^{(E)})$  \label{lst:line:intrasubnet_destination_expression}
         \EndFor
         \State $\texttt{InterSubnet} = ( M^{(E)} \oplus M^{(I)}) \rightarrow ((M^{(E)} \rightarrow R_{subnet}^{(I)}) \wedge ( \lnot M^{(E)} \rightarrow R_{subnet}^{(E)}))$ \label{lst:line:intersubnet_expression}
         \State $R = R \wedge \texttt{InterSubnet} \wedge \texttt{IntraSubnet}$
      \EndFor
      \State \textbf{return} $R$
      \EndProcedure
   \end{algorithmic}
\end{algorithm}

\section{Weighted MaxSAT solution algorithm}\label{app:maxsat}
\cref{alg:wpmres} depicts the main steps of our implementation of the weighted PMRes algorithm. The algorithm receives as input the set of soft constraints to be satisfied which, in our case, is the soft requirement that all of the decision variables remain unassigned, i.e.,  $\omega_i ( \phi_i = \emptyset), \; \forall\phi_i\in(\Phi^{\left(A\right)}\cup\Phi^{\left(D\right)}\cup\ \Psi^{\left(A\right)}\cup\ \Psi^{\left(D\right)})$. The algorithm will try to verify using Z3 wether the current assignment to the constraints satisfies also the hard constraints defined in \cref{eq:intent_satisfaction} and \cref{eq:reachability_conservation} on \cref{{lst:line:checksat}}. If yes the algorithm terminates by returning the current assignment to the decision variables, otherwise some of the soft constraints that make the problem unsolvable undergo a relaxation (\cref{lst:line:relaxwpmres}) procedure, thus allowing the assignment to some of the decision variables. The relaxation procedure will find the soft constraint with the smallest weight that make the problem unsatisfiable (\cref{lst:line:minimum_weight}). The procedure will then permit the assignment of some of the decision variables by removing all of the constraints with the minimum weight (\cref{lst:line:remove_from_constraints}) or and by reducing the cost of the remaining constraints (\cref{lst:line:decrease_weight}). The remainder of the clauses present in the unsatisfiable set will then be transformed to permit a new assignment to some of the clauses by allowing each individual clause to become a soft constraint while keeping the remainder as a hard constraint (\cref{lst:line:clause_relaxation}). Finally the procedure will return the new set of constraint to the main procedure to check for satisfiability.

\begin{algorithm}[t]
   \caption{The implementation of Weighted PMRes algorithm used by VARC for the solution generation}
   \label{alg:wpmres}
   \begin{algorithmic}[1]
      \Procedure{WPMRes}{Constraints, GiveUpThreshold}
      \State $c = \texttt{Constraints}$
         \While{$\texttt{numIterations} < \texttt{GiveUpThreshold}$}
            \State $\texttt{UnsatCore}, \texttt{isSat} = \texttt{checkSAT(Constraints)}$ 
            \If{\texttt{isSat}} \label{lst:line:checksat}
               \State \textbf{return} $c$
            \Else
               \State $c = \texttt{RelaxUnsatCore(}c, \texttt{UnsatCore)}$ \label{lst:line:relaxwpmres}
            \EndIf 
         \State $\texttt{numIterations}{+}{+}$
         \EndWhile
         \State \textbf{return} $\emptyset$
      \EndProcedure
      \\
      \Procedure{RelaxUnsatCore}{Constraints, UnsatCore}
         \State $w_{\texttt{min}} = \infty$ 
         \For{$\texttt{Clause} \in \texttt{UnsatCore}$}
            \State $w_{\texttt{min}} = \texttt{min}(w_{\texttt{min}}, \texttt{Clause.weight})$ \label{lst:line:minimum_weight}
         \EndFor

         \For{$\texttt{Clause} \in \texttt{UnsatCore}$}
            \If{$\texttt{Clause.weight} == w_{\texttt{min}}$}
               \State $\texttt{Constraints} = \texttt{Constraints} \setminus \texttt{Clause}$ \label{lst:line:remove_from_constraints}
            \Else
            \State $\texttt{Clause.weight} = \texttt{Clause.weight} - w_{\texttt{min}}$ \label{lst:line:decrease_weight}
            \EndIf
         \EndFor
         \State $\texttt{AggClause} = \texttt{True}$
         \For{$\texttt{for} \; i = 0, \; i{+}{+}, \; \texttt{while} \; $i <$ \texttt{UnsatCore.size}$} \label{lst:line:clause_relaxation}
            \State $\texttt{RelaxedClause} = \bigwedge_{j=0}^{j<i} \texttt{UnsatCore[j]} \vee \texttt{UnsatCore[i]}$
            \State $\texttt{RelaxedClause.weight} = w_{\texttt{min}}$
            \State $\texttt{Constraints} = \texttt{Constraints} \vee \texttt{RelaxedClause}$
         \EndFor
         \State \textbf{return} \texttt{Constraints}
      \EndProcedure

   \end{algorithmic}
\end{algorithm}
